# Supplementary material for: Explicit Feature Interaction-aware Graph Neural Networks
Source: arXiv:2204.03225 source file (2024-06-13)
Supplement: Supplementary file 1 [file additional_visualization.tex]

\section{Additional Study on Visualization of Feature Interactions}

    We showed that our EFI-GNN is an interpretable AI model and visualized the feature interactions.
    We additionally visualize first-order and second-order feature interactions with different hyper-parameter settings.
    Figure \ref{fig:units}, Figure \ref{fig:layers}, and Figure \ref{fig:seeds} are the visualizations of the first-order feature interactions on the different number of units, layers, and different seeds, respectively.
    The first-order feature interactions have the same trend.
    It indicates that EFI-GNN pays attention to the same features across the different hyper-parameter settings and shows EFI-GNN is reliable.
    Figure \ref{fig:units2} is the visualization of the second-order feature interactions on the different numbers of units.
    Unlike first-order feature interactions, it is hard to find any patterns or trends in second-order feature interactions.
    We anticipate that the node aggregation in an EFI-GNN layer causes this problem.
    An EFI-GNN layer aggregates the features of neighboring nodes.
    This may make it more challenging to capture stable patterns of feature interactions.
    Our future work is to find out exactly why this problem is caused.

    \input{figures/units.tex}
    \input{figures/layers.tex}
    \input{figures/seeds.tex}
    \input{figures/units2.tex}
